# Supplementary material for: Does Reasoning Improve Psychological Depth in Large Language Models? It Depends on Who's Judging
Source: arXiv:2609.13773 source file (2026-09-12)
Supplement: Supplementary file 2 [file Agreement.tex]

\section{Additional agreement analyses}
\label{app:agreement}
Table~\ref{tab:iaa_breakdown} shows the inter-annotator agreement breakdown of each model pair. The near-zero and occasionally negative agreement scores highlight the subjective variance present across all frontier model matchups, regardless of reasoning budget or architecture.

\label{app:iaa_breakdown}
\begin{table}[t]
\caption{Krippendorff's $\alpha$ inter-annotator agreement broken down by specific model pairing. Bold indicates the highest value among dimensions in each column.}
\label{tab:iaa_breakdown}
\centering
\small
\begin{tabular}{lcccc}
\toprule
\textbf{Metric} & \textbf{Overall $\alpha$} & \textbf{DeepSeek-R1 vs V3} & \textbf{GPT-5 (auto) vs 4o} & \textbf{GPT-5 (high) vs 4o} \\
\midrule
Authenticity & 0.037 & 0.073 & 0.053 & $-0.015$ \\
Emotion Prov. & 0.082 & 0.035 & 0.147 & 0.072 \\
Empathy & \textbf{0.185} & 0.047 & \textbf{0.176} & \textbf{0.290} \\
Engagement & 0.061 & \textbf{0.101} & 0.010 & 0.080 \\
Narr.\ Complexity & 0.018 & 0.049 & $-0.013$ & 0.005 \\
Preference & 0.038 & 0.074 & $-0.003$ & 0.050 \\
\midrule
\textbf{Average} & 0.070 & 0.063 & 0.062 & 0.080 \\
\bottomrule
\end{tabular}
\end{table}

Figure~\ref{fig:auto_agreement} shows the agreement between the LLM-as-Judge evaluator and human majority vote, broken down by model pair and PDS dimension.

\begin{figure}[t]
\centering
\includegraphics[width=\linewidth]{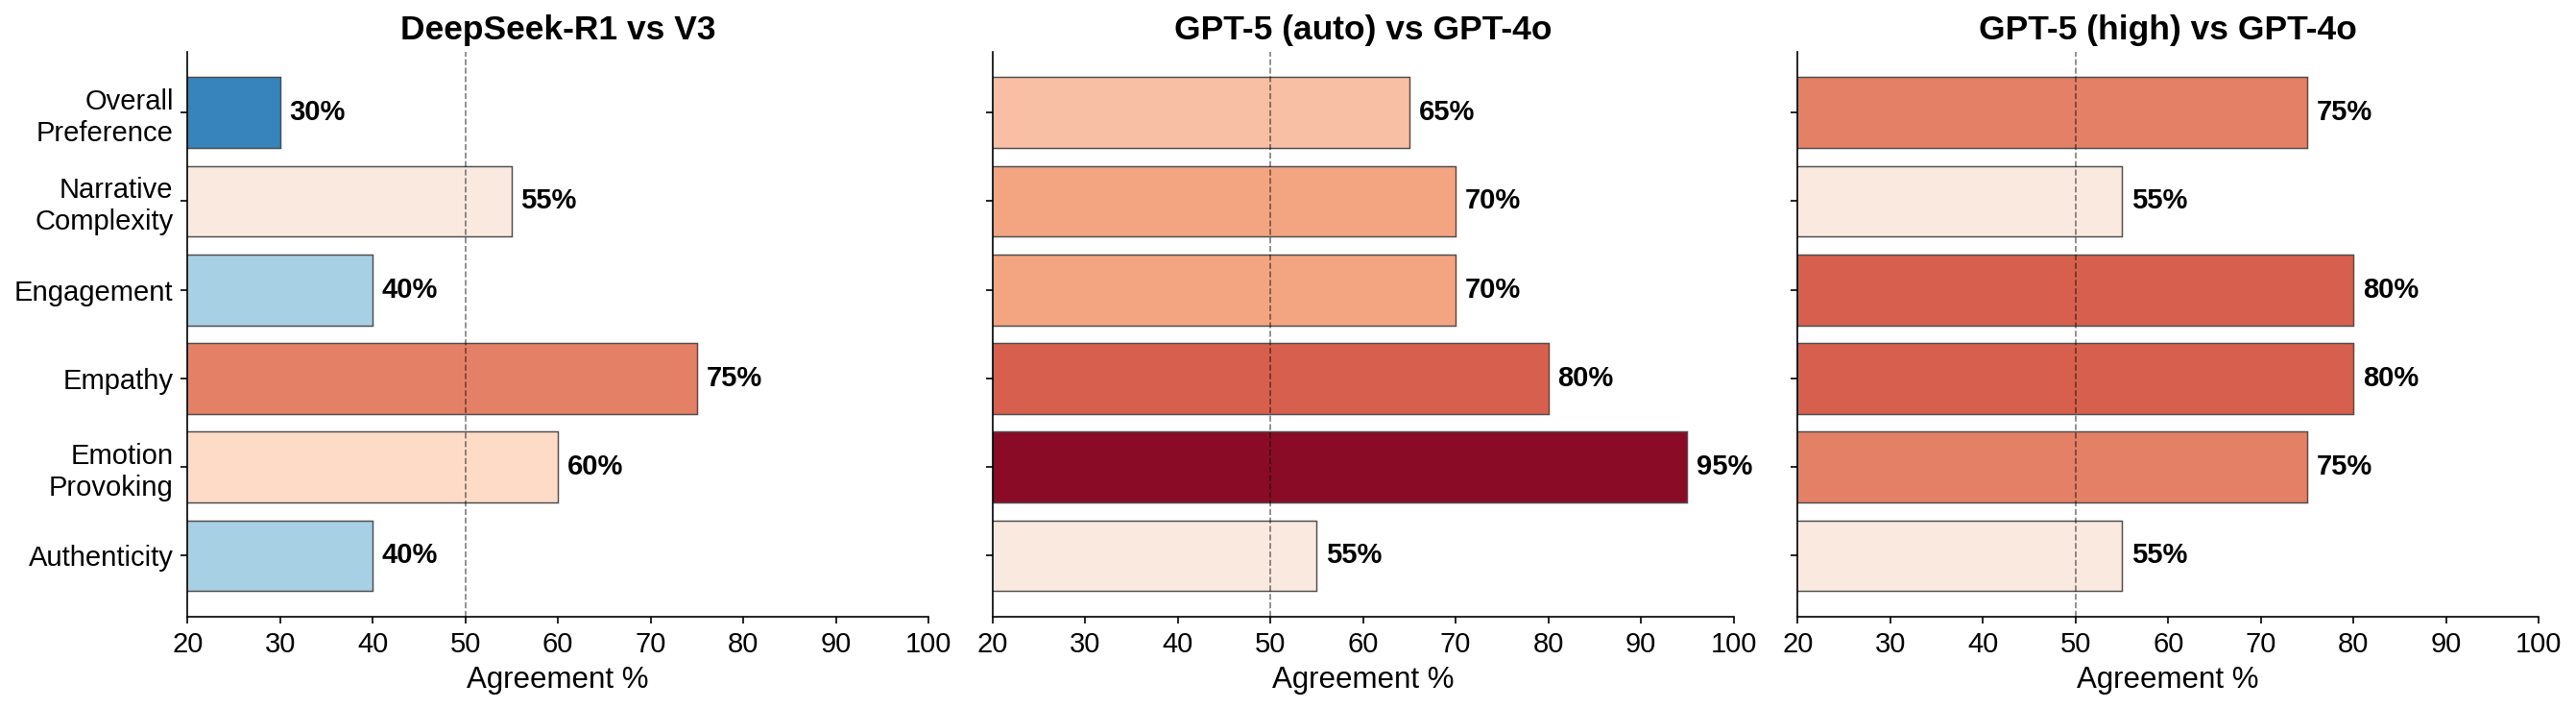}
\caption{Agreement between the LLM-as-Judge evaluator and human majority vote by model pair. The dashed line indicates chance ($50\%$).}
\label{fig:auto_agreement}
\end{figure}
