# Supplementary material for: Does Reasoning Improve Psychological Depth in Large Language Models? It Depends on Who's Judging
Source: arXiv:2609.13773 source file (2026-09-12)
Supplement: Supplementary file 8 [file Single_Judge.tex]

\section{Individual judge preference rates}
  \label{sec:appendix-judge-breakdown}    
  Table~\ref{tab:judge_breakdown} reports the preference rate for the reasoning model for each individual judge configuration in the ensemble, expressed as strict wins out of decisive pairs (ties excluded). All five judges exhibit a consistent pro-reasoning bias across all PDS dimensions, confirming that the ensemble's 98.3\% overall preference is not driven by any single judge. Asterisks indicate the dimension for which each judge was selected in the ensemble.    
  The rightmost column reports the total number of tied pairs (out of 300 judge--dimension cells).    
  \begin{table}[t]
  \caption{Individual judge preference rates for the reasoning model across all 60 pairs, reported as strict wins\,/\,decisive pairs (ties excluded). $^*$~denotes the dimension routed to that judge; it does not denote the highest preference rate. The Avg column is the mean win rate across the five dimensions.}
  \label{tab:judge_breakdown}
  \centering
  \small                         
  \begin{tabularx}{\linewidth}{X ccccc cc}
  \toprule
  \textbf{Judge} & \textbf{Auth.} & \textbf{Emo.} & \textbf{Emp.} & \textbf{Eng.} & \textbf{Narr.} & \textbf{Avg} & \textbf{Ties} \\          
  \midrule                          
  Llama 3.1 70B (5d)  & 43/44$^*$ & 54/57 & 49/54 & 47/51 & 53/55 & 94.3\% & 39 \\
  Llama 3.1 70B (10d) & 43/43 & 53/53$^*$ & 48/51 & 46/46 & 54/54 & 98.8\% & 53 \\
  Llama 3.3 70B (10d) & 32/33 & 53/55 & 51/57$^*$ & 47/58 & 47/56 & 89.6\% & 41 \\
  Qwen3.5 397B (7d)   & 57/57 & 58/58 & 55/58 & 57/59$^*$ & 57/58 & 97.9\% & 10 \\
  Llama 3.1 70B CoT   & 7/8 & 49/50 & 47/53 & 43/55 & 49/59$^*$ & 87.1\% & 75 \\
  \midrule                          
  \textbf{Ensemble}    & 43/44 & 53/53 & 51/57 & 57/59 & 49/59 & 93.4\% & 28 \\
  \bottomrule                      
  \end{tabularx}
  \end{table}  
