# Supplementary material for: Does Reasoning Improve Psychological Depth in Large Language Models? It Depends on Who's Judging
Source: arXiv:2609.13773 source file (2026-09-12)
Supplement: Supplementary file 9 [file Tie_Break.tex]

\section{Tie-breaking statistics for the ensemble evaluator}
\label{sec:appendix-ties}

When the ensemble evaluator assigns identical Likert scores to both stories on a
given dimension, the tie is broken by random assignment. Table~\ref{tab:ties}
reports the number of ties per dimension across all 60 pairs. Ties occur rarely on most dimensions. The headline
98.3\% preference rate involves zero ties. Even on authenticity, where ties are
most frequent, the pro-reasoning bias among decisive pairs remains near-ceiling.

\begin{table}[t]
\caption{Tie frequency and decisive-pair outcomes for the ensemble evaluator.}
\label{tab:ties}
\centering
\small
\begin{tabular}{l cc c}
\toprule
\textbf{Dimension} & \textbf{Ties} & \textbf{Decisive} & \textbf{Reasoning wins (decisive)} \\
\midrule
Authenticity       & 16 & 44 & 43 (97.7\%) \\
Emotion Prov.      & 7  & 53 & 53 (100.0\%) \\
Empathy            & 3  & 57 & 51 (89.5\%) \\
Engagement         & 1  & 59 & 57 (96.6\%) \\
Narr.\ Complexity  & 1  & 59 & 49 (83.1\%) \\
\midrule                          
Preference         & 0  & 60 & 59 (98.3\%) \\
\bottomrule
\end{tabular}
\end{table}
