# Supplementary material for: Does Reasoning Improve Psychological Depth in Large Language Models? It Depends on Who's Judging
Source: arXiv:2609.13773 source file (2026-09-12)
Supplement: Supplementary file 10 [file appendix.tex]

\clearpage
\appendix
\input{content_v2/Appendix/Premises}
\input{tables/all_premises}

\input{content_v2/Appendix/Generation}

\input{content_v2/Appendix/Tie_Break}

\input{content_v2/Appendix/Agreement}

\input{content_v2/Appendix/Annotation}

\clearpage

\input{content_v2/Appendix/Comment}

\input{content_v2/Appendix/Single_Judge}

\input{content_v2/Appendix/Heatmaps}

\input{content_v2/Appendix/Case_Study}
